# Supplementary material for: Auditing and Debugging Deep Learning Models via Decision Boundaries: Individual-level and Group-level Analysis
Source: arXiv:2001.00682 source file (2020-01-03)
Supplement: Supplementary file 1 [file Appendix_D.pdf]

# D HOMOTOPY ALGORITHM FOR COMPUTING FLIP POINTS

**General approach.** If the activation function is differentiable (e.g., erf), we can make use of its gradient in solving the optimization problems we have introduced. Otherwise, subgradients can be used, but this can make the optimization algorithms more costly.

The gradient of the outputs of the network with respect to its inputs is a Jacobian matrix when the network has more than one input feature and more than one output class. We compute this gradient analytically, which is generally more efficient and reliable than using finite differences. Analytic computation of the gradients is possible for many different kinds of network architectures, including feed-forward, convolutional, and residual networks, assuming that the network does not contain non-differentiable elements such as non-differentiable activation functions or max pooling.

For the feed-forward networks used in this work, the computation of the gradient is analogous to the back-propagation approach commonly used to compute the gradients with respect to the training parameters of the networks [30].

Using the gradients, we minimize (1) subject to the constraints mentioned in Section 3 in order to find the closest flip point. The problem is non-convex, so standard optimization software generally computes a local minimizer but not necessarily a global minimizer. In the case of inputs with discrete features, we can add the discrete constraints to the problem or add regularization terms to the objective function using the techniques described by Nocedal and Wright [23].

Our optimization problem can be considered a generally solvable problem using off-the-shelf methods available in the literature. However, difficulties sometimes arise in solving nonlinear non-convex optimization problems, and therefore it is beneficial to design an optimization method tailored to our particular problem. To illustrate this, we first specify our network and then our optimization algorithm.

In our notation, vectors and scalars are in lower case and matrices are in upper case. Bold characters are used for vectors and matrices, and the relevant layer in the network is shown as a superscript in parenthesis. Subscripts denote the index for a particular element of a matrix or vector. Iterations of the algorithm are denoted by superscripts.

**Our neural network.** We specify the neural network $\mathcal{N}$ shown in Figure D1 by weight matrices $\boldsymbol{W}^{(k)}$ and bias vectors $\boldsymbol{b}^{(k)}$ for each layer $k = 1, \ldots, m$. The output of layer $k$ in the network is denoted by $\boldsymbol{y}^{(k)}$.

The activation function used in the nodes is the error function

$$y = activation(c|\sigma) = \text{erf}(\frac{c}{\sigma}) = \frac{1}{\sqrt{\pi}} \int_{-\frac{c}{\sigma}}^{+\frac{c}{\sigma}} e^{-t^2} dt,$$

where $c$ is the result of applying the weights and bias to the node's inputs. The tuning parameter $\sigma$ is constant among the nodes on each layer and is optimized during the training process. Hence, for the whole network, we have a vector of tuning parameters, $\boldsymbol{\sigma}$, where each element of it corresponds to one hidden layer in the network. While erf is not a very common choice for activation function, it has been shown that its performance in terms of accuracy is comparable to other activation functions [24]. We note that when $\sigma$ is small, then the activation function resembles a step function, while when $\sigma$ is large, it resembles a linear function, as shown in Figure D2, so erf captures the behavior of popular activation functions while preserving differentiability.

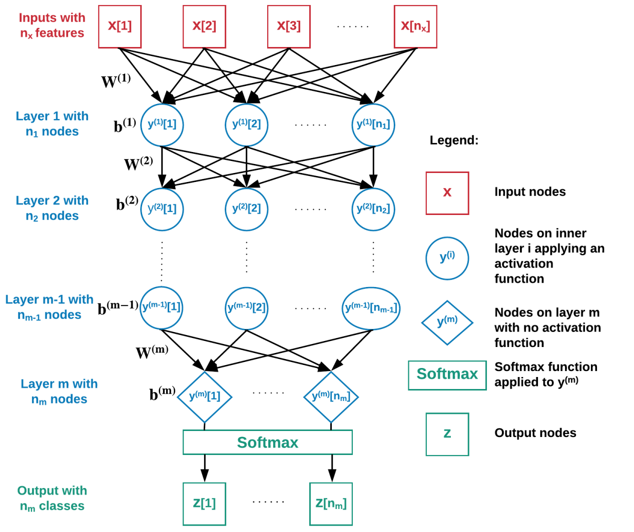


**Figure D1: Sketch of a prototype feed-forward neural network $\mathcal{N}$ with $n_x$ inputs, $m$ layers, and $n_m$ outputs.**

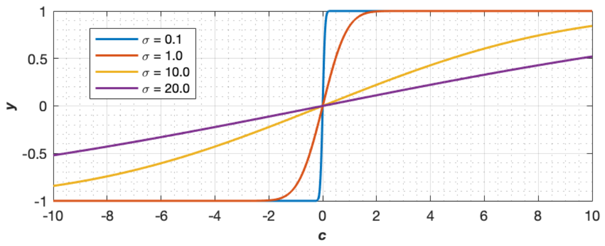


**Figure D2: Shape of erf function as $\sigma$ varies.**

Using the erf activation function, the output of the first inner layer for input $\boldsymbol{x}$ is

$$\boldsymbol{y}^{(1)} = \text{erf}\left(\frac{\boldsymbol{x}\boldsymbol{W}^{(1)} + \boldsymbol{b}^{(1)}}{\sigma_1}\right).$$

For the hidden layers,

$$\boldsymbol{y}^{(i)} = \text{erf}\left(\frac{\boldsymbol{y}^{(i-1)}\boldsymbol{W}^{(i)} + \boldsymbol{b}^{(i)}}{\sigma_i}\right).$$

Finally,

$$\boldsymbol{y}^{(m)} = \boldsymbol{y}^{(m-1)}\boldsymbol{W}^{(m)} + \boldsymbol{b}^{(m)},$$

and the output of the network is

$$\boldsymbol{z}(\boldsymbol{x}) = \text{softmax}\left(\boldsymbol{y}^{(m)}\right).$$

**Optimization framework.** We recommend a homotopy method for calculating the closest flip points. Here, we briefly explain its framework in the context of our network. Our method can be easily generalized to neural networks with different architectures, such

as convolutional and residual networks. The homotopy algorithm applies an optimization module to a series of networks.

**Optimization module.** We define the numerical process of computing the closest flip point $\hat{x}^c$ to an input $\boldsymbol{x}$ between classes $i$ and $j$ by the function $\mathcal{F}$:

$$\hat{\mathbf{x}}^c{}_{(i,j)} = \mathcal{F}(\boldsymbol{x}, \mathcal{N}, \mathbf{x_0}, C, i, j),$$

We assume $\mathcal{F}$ is a standard off-the-shelf optimizer. The inputs to $\mathcal{F}$ include the trained neural network $\mathcal{N}$, the starting point $\mathbf{x_0}$, and the constraints $C$. As a general practice and based on our numerical experiments, an interior-point algorithm can be considered a good choice, as it is known to be successful in solving constrained, non-linear, non-convex optimization problems with high dimensional variables [23]. This can be used in conjunction with a branch-and-bound algorithm for discrete variables.

Ideally, $\mathcal{F}$ efficiently finds the closest flip point for our network, possibly using the input $\boldsymbol{x}$ as the starting point. If this fails, then we use a *homotopy method*, starting by applying $\mathcal{F}$ to an easier network and gradually transforming it to the desired network, each time using the previously determined flip point as our starting point for $\mathcal{F}$. We now discuss the family of networks used in the homotopy.

**Homotopy algorithms.** Our homotopy method, defined by Algorithm D1, begins with a neural network for which $\boldsymbol{x}$ is a flip point, and then computes flip points for a series of networks, gradually transforming to the original network, using the closest flip point found at each iteration as the starting point for the next iteration. This way, the algorithm follows a path of flip points starting from $\boldsymbol{x}$, until it finds the closest flip point to $\boldsymbol{x}$ for the original network.

**Algorithm D1** Homotopy algorithm for calculating closest flip point

**Inputs**: $\mathcal{N}$, $\boldsymbol{x}$, $\eta$, $\tau$, $C$, $i$, $j$
**Output**: Closest flip point to $\boldsymbol{x}$

1: Compute $\boldsymbol{\sigma}^h$ and $\boldsymbol{b}^{h(m)}$ using Algorithm D2 with inputs ($\mathcal{N}$, $\boldsymbol{x}$, $\tau$, $i$, $j$)
2: $\hat{\mathbf{x}}^{c,0} = \boldsymbol{x}$
3: **for** $k = 1$ to $\eta$ **do**
4: $\quad \boldsymbol{\sigma}^k = \boldsymbol{\sigma}^h + k(\frac{\boldsymbol{\sigma}^{\mathcal{N}} - \boldsymbol{\sigma}^h}{\eta})$
5: $\quad \boldsymbol{b}^{k(m)} = \boldsymbol{b}^{h(m)} + k(\frac{\boldsymbol{b}^{\mathcal{N}(m)} - \boldsymbol{b}^{h(m)}}{\eta})$
6: $\quad$ Replace $\boldsymbol{\sigma}^k$ and $\boldsymbol{b}^{k(m)}$ in $\mathcal{N}$, to obtain $\mathcal{N}^k$
7: $\quad \hat{\mathbf{x}}^{c,k} = \mathcal{F}(\boldsymbol{x}, \mathcal{N}^k, \hat{\mathbf{x}}^{c,k-1}, C, i, j)$
8: **end for**
9: **return** $\hat{\mathbf{x}}^{c,\eta}$ as the closest flip point to $\boldsymbol{x}$

The initial neural network used in the algorithm is the same as the original network except that it has parameters $\boldsymbol{\sigma}^h$ for the erf and $\boldsymbol{b}^{h(m)}$ for the bias on the last layer. These are computed in Algorithm D2, discussed below.

The parameter $\eta$ defines the number of iterations that Algorithm D1 uses to transform the network back to its original form. A large $\eta$ means that each neural network is a small change from the previous one, so the starting point is close to the solution. A small $\eta$ means that only a few optimization problems are solved, but each starting point may be far from the solution. We want to perform enough iterations so that the global minimizer is found, but we also want

**Algorithm D2** Algorithm to transform the network for the Homotopy algorithm

**Inputs**: $\mathcal{N}$, $\boldsymbol{x}$, $\tau$, $i$, $j$
**Output**: $\boldsymbol{\sigma}^h$ and $\boldsymbol{b}^{h(m)}$

1: $\gamma = \sqrt{log(\frac{2}{\tau\sqrt{\pi}})}$
2: $\boldsymbol{y}^{(0)} = \boldsymbol{x}$
3: **for** $k = 1$ to $m-1$ **do**
4: $\quad \sigma^h_k = \max(\frac{2}{\sqrt{\pi}}, \frac{1}{\gamma} \|\boldsymbol{y}^{(k-1)}\boldsymbol{W}^{(k)} + \boldsymbol{b}^{(k)}\|_\infty)$
5: $\quad$ **if** $\sigma^h_k > \frac{2}{\tau\sqrt{\pi}}$ **then**
6: $\quad\quad \boldsymbol{c} = \boldsymbol{y}^{(k-1)}\boldsymbol{W}^{(k)} + \boldsymbol{b}^{(k)}$
7: $\quad\quad$ **for** $t = 1$ to $n_k$ **do**
8: $\quad\quad\quad \sigma^h_{k,t} = \max(\frac{2}{\sqrt{\pi}}, \frac{1}{\gamma} c_t)$
9: $\quad\quad$ **end for**
10: $\quad$ **end if**
11: $\quad \boldsymbol{y}^{(k)} = \text{erf}(\frac{\boldsymbol{y}^{(k-1)}\boldsymbol{W}^{(k)} + \boldsymbol{b}^{(k)}}{\sigma^h_k})$
12: **end for**
13: $\min_{\boldsymbol{b}^{h(m)}} \|\boldsymbol{b}^{h(m)} - \boldsymbol{b}^{\mathcal{N}(m)}\|_2$ , subject to:
$\quad$ (1) $\boldsymbol{y}^{(m)} = \boldsymbol{y}^{(m-1)}\boldsymbol{W}^{(\boldsymbol{m})} + \boldsymbol{b}^{h(m)}$,
$\quad$ (2) $y^{(m)}_i = y^{(m)}_j$,
$\quad$ (3) $\forall\ l \neq i, j \mid y^{(m)}_i > y^{(m)}_l$
14: **return** $\boldsymbol{\sigma}^h, \boldsymbol{b}^{h(m)}$

to keep the computational cost low. We have achieved best results with $\eta$ ranging between 1 and 10. Choosing $\eta = 1$ is equivalent to not using the homotopy algorithm and directly applying $\mathcal{F}$ to the original network with starting point $\boldsymbol{x}$.

The initial transformation of the network is performed by Algorithm D2, pursuing two goals, first, bounding the flow of gradients through the layers of the network by changing the value of tuning parameters (lines 1 through 12), and second, changing the bias parameters in the last layer of the network so that $\boldsymbol{x}$ is a flip point for the transformed network (line 13).

The tuning parameters for the original network are $\boldsymbol{\sigma}^{\mathcal{N}}$, and $\boldsymbol{\sigma}^h$ denotes the transformed parameters computed by Algorithm D2. Similarly, $\boldsymbol{b}^{\mathcal{N}(m)}$ and $\boldsymbol{b}^{h(m)}$ denote the original and transformed bias in the last layer of the network.

By changing $\boldsymbol{\sigma}^{\mathcal{N}}$ to $\boldsymbol{\sigma}^h$, we try to control the magnitudes of the gradients of output with respect to inputs. The hierarchy of neural networks can cause the gradients to vanish and/or explode through its layers, which could lead to a badly scaled gradient matrix and eventually an ill-conditioned optimization problem, and we would like to avoid this. For flip point computation, we are concerned about the gradients of outputs with respect to inputs, while in neural network literature, this issue of "vanishing and exploding gradients" usually concerns the training process and the gradient of the loss function with respect to the training parameters [1, 10]. In both cases, the "vanishing and exploding gradients" phenomenon can be studied by investigating individual matrices in the chain rule formulation of the gradient matrix.

To compute the $\boldsymbol{\sigma}^h$, we trace the $\boldsymbol{x}$ as it flows through the layers of the network. As the input reaches each hidden layer, before applying the activation function, we tune the corresponding element of $\boldsymbol{\sigma}^h$, so that the absolute values of the gradients of the output of each neuron, with respect to neuron's input, is greater than or equal to $\tau$, and less than or equal to 1. In our numerical experiments, we have used different values of $\tau$ ranging between $10^{-5}$ and $10^{-9}$.

In Algorithm D2, line 1 computes a scalar $\gamma$ such that the derivative of the erf is equal to $\tau$. Lines 3 through 12, tune the $\sigma$, layer by layer, starting from the first layer and ending at the last hidden layer. Line 4 bounds the individual gradient between $\tau$ and 1. Choosing the $\sigma_k^h > \frac{2}{\sqrt{\pi}}$ ensures the gradients of neurons are upper bounded by 1. This relationship can be easily derived by setting the maximum derivative of erf equal to $\tau$.

Choosing $\sigma_k^h \geq \frac{1}{\gamma} \|\boldsymbol{y}^{(k-1)}\boldsymbol{W}^{(k)} + \boldsymbol{b}^{(k)}\|_\infty$ can potentially make the gradients of all the neurons in layer $k$ lower bounded by $\tau$. Sometimes, this might not be possible to achieve for all the neurons in a layer, if we obtain $\sigma_k^h > \frac{2}{\tau\sqrt{\pi}}$. In such situations, we calculate the $\sigma_k^h$ separately for each neuron on that layer (lines 5 through 10), and use a non-uniform $\sigma_k^h$ in the homotopy algorithm. Line 11, computes the output of each layer after the $\sigma$ is tuned for that layer.

Since our activation function is erf, we can effectively control the gradients and make them bounded. The maximum gradient of erf is at point zero, and by moving away from zero, its gradient decreases monotonically, until it asymptotically reaches zero. This boundedness and the monotonicity of both the erf and its gradient are helpful features that we leverage in our homotopy method. When using activation functions other than erf, we have to avoid exploding and vanishing gradients, depending on the properties of the activation function in use.

By changing $\boldsymbol{b}^{\mathcal{N}(m)}$ to $\boldsymbol{b}^{h(m)}$, computed at line 13 of Algorithm D2, the input $\boldsymbol{x}$ actually becomes a flip point for the transformed network. Having a starting point that is feasible with respect to flip point constraints considerably facilitates the optimization process. The optimization problem on line 13 of the algorithm is a convex quadratic programming problem and can be solved by standard algorithms.
